# Supplementary material for: Distributional Dataset Distillation with Subtask Decomposition
Source: arXiv:2403.00999 source file (2024-03-01)
Supplement: Supplementary file 1 [file appdx_ablation.tex]

\section{Additional Ablation Study}
\subsection{Loss function contribution}
\label{apdx:loss_term}
To understand the contribution of each loss terms, we repeat Algo.~\ref{algo:main} to performance distillation on CIFAR-10 with subsets of different loss terms. Table \ref{tab:loss_term_1} exhibits test performance of 1 PPC and Table~\ref{tab:loss_term_2} exhibits test performance for 2 PPC, where there is an additional diversity term in the loss function. Both tables indicate that MTT loss generate distributions that work well on seen architecture, but fail to generalize to new architectures. On the other hand, DM loss generates distributions that generalize well to unseen architectures but overall converge to a lower distillation quality. The sub-par performance for DM on seen architecture is more prominent at higher PPC case, as reflected in Table~\ref{tab:loss_term_2}. However, our when we use MTT and DM together, the distilled distributions show a clear improvement from both loss terms alone. Table~\ref{tab:loss_term_ipc} shows that diversity loss contributed to a small but consistent increase in the overall distillation quality. 

\begin{table}[ht]
\caption{Results (Test Accuracy$\%$) of ablation study on the contribution of each loss terms at 1 PPC scenarios using CIFAR-10}
\centering
% \resizebox{0.6\textwidth}{!}{
    \begin{tabular}{@{\extracolsep{4pt}}lcccc}
    \toprule   
    {} & \multicolumn{4}{c}{\textbf{Evaluation Model}} \\
     \cmidrule(lr){2-5} 
     \textbf{Loss Terms Used}  & ConvNet & ResNet18 & VGG11& AlexNet \\ 
     \midrule
          DM & \errbar{57.4}{0.23} & \errbar{48.1}{0.33} & \errbar{42.6}{0.12} & \errbar{35.6}{0.43} \\
          MTT & \errbar{56.5}{0.22} & \errbar{43.7}{0.15} & \errbar{48.6}{0.2} & \errbar{27.7}{0.22}\\ 
          MMT and DM& \errbar{61.2}{0.14} & \errbar{56.5}{0.35} & \errbar{53.5}{0.47} & \errbar{42.4}{0.68} \\
    \bottomrule
    \end{tabular}
    % }
\label{tab:loss_term_1}
% \end{table}

% \begin{table}[ht]
    % \begin{minipage}[t]{0.5\textwidth}
    \caption{Results (Test Accuracy$\%$) of ablation study on the contribution of each loss terms at 2 PPC scenarios using CIFAR-10}
    \centering
    % \resizebox{\textwidth}{!}{
        \begin{tabular}{@{\extracolsep{4pt}}lcccc}
        \toprule   
        {} & \multicolumn{4}{c}{\textbf{Evaluation Model}} \\
         \cmidrule(lr){2-5} 
         \textbf{Loss Terms Used}  & ConvNet & ResNet18 & VGG11& AlexNet \\ 
         \midrule
              DM & \errbar{55.6}{0.34} & \errbar{44.9}{0.62} & \errbar{43.9}{0.30} & \errbar{42.4}{0.66} \\
              MTT & \errbar{61.5}{0.22} & \errbar{47.3}{0.47} & \errbar{47.6}{0.29} & \errbar{27.6}{0.50}\\ 
              MMT, DM& \errbar{63.1}{0.51} & \errbar{57.5}{0.39} & \errbar{55.5}{0.22} & \errbar{45.2}{0.24} \\
              % MMT, DM, Diversity & \errbar{64.98}{0.14} & \errbar{61.07}{0.30} & \errbar{59.50}{0.53} & \errbar{51.80}{1.80}\\
        
        \bottomrule
        \end{tabular}
        % }
    \label{tab:loss_term_2}
\end{table}
% \end{minipage}
% \begin{minipage}[t]{0.5\textwidth}

% \subsection{Number of latent priors per class}
