# Supplementary material for: Distributional Dataset Distillation with Subtask Decomposition
Source: arXiv:2403.00999 source file (2024-03-01)
Supplement: Supplementary file 2 [file appdx_related.tex]

\section{Additional Related Work}
\paragraph{Data Factorization.} In contrast to all methods listed so far, data factorization approaches distill data in a latent space \citep{deng2022remember,liu2022datset}. For downstream tasks, a decoder (generator)  maps the base vectors to the data space on-demand. The advantage of introducing the decoder is to allow mutual information shared by distilled examples. LinBa (\cite{deng2022remember}) generates a data point using a linear combination of all the bases, while HaBa (\cite{liu2022datset}) generates a data sample using a single base vector. IDC \citep{kim2022dataset} stores a down-sampled version of synthetic images and conducts bi-linear upsampling in downstream training, while KFS (\cite{leehb2022dataset}) uses class-based latent vectors and multiple decoders to generate data.

\paragraph{Generative Distillation.} This line of work learns the latent code and uses pre-trained GANs as the decoder to output training images. GLaD (\cite{cazenavette2023generalizing}) extends MTT, and shows that optimizing in latent space promotes better cross-architecture generalizability. Building on DM (\cite{zhao2023dataset}), IT-GAN \cite{zhao2022synthesizing} learns a distinct latent code for every sample in the training set with the help of GAN Inversion.
